# Supplementary material for: A Two-Stage Method for Chinese AMR Parsing
Source: arXiv:2209.14512 source file (2022-09-29)
Supplement: Supplementary file 1 [file appendix.tex]

# Normalization Alignment case
1. Concepts that need to add a word sense number
这 几 天 关于 中 俄 战略 合作 伙伴 关系 成 了 大 热点 。
'合作'->'合作-01', '成'->'成-01', '大'->'大-01'

2. Concepts that need to be transformed to a proper word
但 大 方向 不 会 变 ， 他 就 在 那里 。
'不'->'-', '在'->'be-located-at-91'

3. Concepts that need to be transformed to a number
第一 ， 可以 有效 牵制 美国 对 中国 的 打压 。
'第一'->'1'

4. Concepts that require error correction
那些 JY 一 听 我 说 ， 美国 不 是 为了 民主 ， 而 是 为了 利益 。
'JY' -> '精英'

5. Concepts that require error correction and add a word sense number
闹 得 轰轰扬扬 沸腾 一时 的 合肥 中学 “ 少女 毁容 案件 ” ， 随着 媒体 暴光 大众 关注 有 新 进展 。
'暴光'-> '曝光-01'

# How to generate tag for None Alignment concept.
1. 从训练集中总结出现的非对齐概念，总共184个 
2. 定义输入序列的触发词 最前或最后 最后：实验证明效果更好
3. 当没有触发词时，即非对齐概念触发非对齐概念。
Since there is no dictionary of all non-aligned concepts, we use all non-aligned concepts that appear in the training set as labels for sequence tagging. Statistically, a total of 184 non-aligned concepts appear in the training set. 
For all non-aligned concepts, we need to define its trigger words. There are two types of trigger words in the training set. The first one are concepts other than non-aligned concepts, that is, we can find a specific trigger word from the sentence. The other one are non-aligned concepts, that is, we cannot find a specific trigger word from the sentence. For example, "and" is triggered by "country" and "country", where "country" is a non-aligned concept triggered by other words.
For both of these trigger cases, there are multiple concepts that can be related to the target concept. Our approach is to first deal with the case where a concept in a sentence triggers a non-aligned concept. To make the tagging process more regular, we tried using the first and the last of the multiple concepts related to the target concept. The experimental results show that using the last concept is more effective. After that we deal with the case where the non-aligned concept triggers the non-aligned concept. We keep going back from the AMR graph of this sentence until we get back to the first concept present in the sentence and use it as the triggering concept.

# WSD rules
We design a set of word sense disambiguation rules to handle concepts that need to be normalized. As listed in appendix A, there are five categories of concepts that need to be normalized. For the 3rd categories, namely, concepts that need to be converted into numbers, we extract the numbers in a sentence using regular expressions, and then convert the numbers into Arabic numerals. For the 4th and 5th categories of concepts, we retrieve the most similar words in the dictionary which is provided based on the phonological and calligraphical code of Chinese character, and then return the corresponding concepts for error correction purposes. For the other cases, we directly use the concept that appears most frequently in the training set.

When we simply use the concepts that appear most frequently in the training set, the accuracy on the development set is 85.1. When we incorporated the above rules, the accuracy increased to 90.6, proving that the rules we designed can effectively handle a number of normalized concepts.

As shown in Table~\ref{tab:norm cases}, we mainly summarize 4 cases that require word normalization. The Word Sense Disambiguation case denotes that the concept is required to select a word sense in terms of its semantic. In table 3, "合作" is interpreted as the No.1 meaning in the dictionary, so "合作" should become "合作-01". The Special Concept Transform case is that many concepts with similar semantics in the corpus are replaced by special token. For example, "不" and "否" are replaced by "-". The Number Normalization case is that all concepts containing numbers need to be converted to Arabic numerals. The Error Correction case denotes that there may be errors in the sentence and we need to correct it according to the dictionary.
